# Supplementary material for: Domain-Wall Ferroelectric Polarons in a two-dimensional Rotor Lattice Model
Source: arXiv:2407.19993 source file (2025-01-03)
Supplement: Supplementary file 1 [file supplement.pdf]

# Supplemental Material for "Domain-Wall Ferroelectric Polarons in a two-dimensional Rotor Lattice Model"

## CONTENTS


I. Introduction 1

II. Structural symmetry breaking and pseudo-Jahn-Teller effect 2

III. Dirac-Frenkel variational principle 3

IV. Variational localized ansatz 4

V. Pseudo Lang-Firsov transformation in the strong coupling regime 5

VI. Classical treatment of the rotors 6

VII. Variational polaron ansatz in the co-moving frame 9

VIII. Perturbation Theory in the weak coupling regime 9

IX. Comparison of the variational methods 10

References 11


## I. INTRODUCTION

In this supplemental material, we present the details of two variational and two perturbative calculations that support the physical findings presented in the main text. In Part II, we discuss the expansion of the electron kinetic energy up to second order in the tunneling anisotropy $\Delta_t$. This expansion counteracts the structural instability that arises from the rotor-electron coupling and thus leads to the definition of a critical lattice stiffness, which is the main finding of our work. In Part III, we provide a detailed account of the Dirac-Frenkel variational principle that we employ to obtain the ground state energies and wavefunctions for the two variational ansätze. In Parts IV and V, we present the mean-field localized ansatz and the pseudo Lang-Firsov transformation, respectively. The latter serves to validate the variational localized ansatz in the strong-coupling limit. In Part VI, we discuss a classical treatment of the rotors, which further validates the variational results in the intermediate coupling regime. In Parts VII and VIII, we present a variational polaron ansatz in the co-moving frame of the electron (vGH ansatz), and a Brillouin-Wigner perturbation calculation in the weak-coupling limit, respectively. Once more, the perturbative calculation is employed to corroborate the polaron ansatz in the weak coupling limit. Moreover, in Part IX, we compare the energies and phase diagrams of both variational approaches and the semiclassical calculation in the $\Delta_t$–$V_0$ plane.

## II. STRUCTURAL SYMMETRY BREAKING AND PSEUDO-JAHN-TELLER EFFECT

In order to provide a concrete example regarding the structural instability in the electron lattice due to the rotor-electron coupling as presented in the main text, in this section we construct a model for such a process.

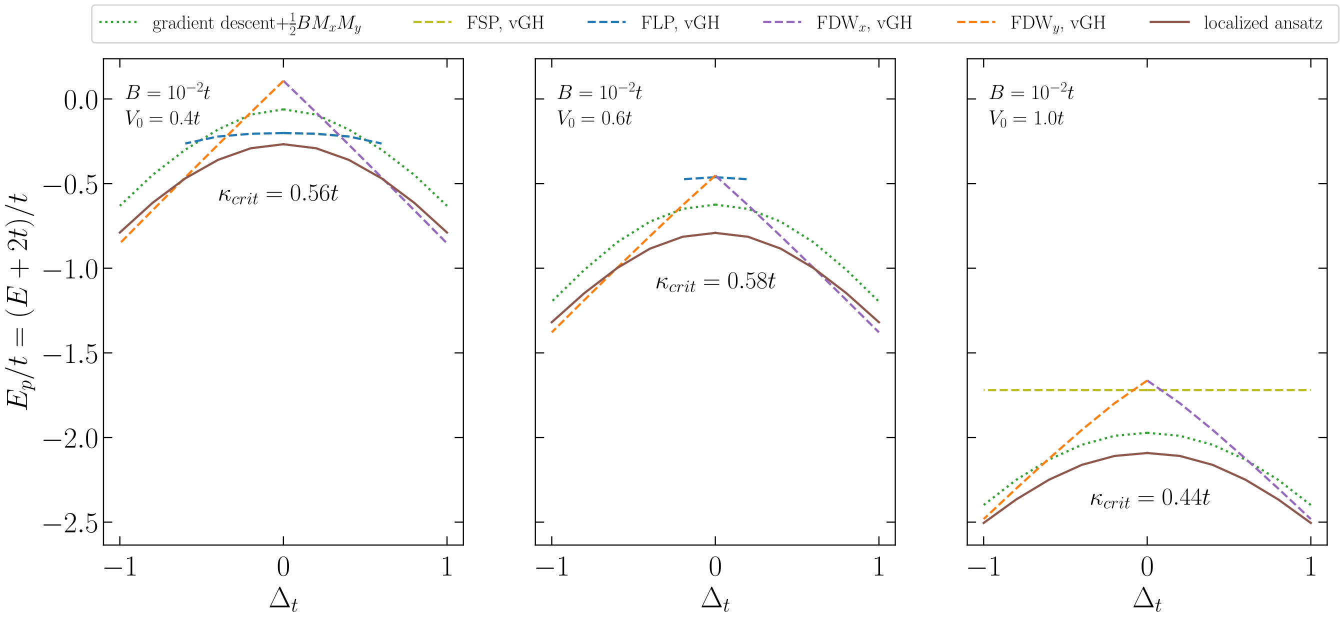


FIG. 1. Dependence of the energy on the tunneling asymmetry parameter $\Delta_t$ for three different coupling strengths, $V_0/t = 0.4, 0.6$ and 1.0, $B = 10^{-2}t$. We also give the values for the critical lattice stiffness, $\kappa_{\text{crit}}$, which lead to the stability-instability phase diagram in Fig. 4(b) of the main text. The dashed lines correspond to the energies obtained within the vGH ansatz and the solid lines show the energies obtained within the localized ansatz. The green dotted lines show the energies obtained from a semiclassical gradient descent calculation, corrected by the rotor self-energy, $BM_xM_y/2$ (here $M_x = M_y = 10$). The calculation of the classical energies is described in section VI.

*Instability Condition.* We start by introducing lattice distortions in the electron lattice. The electron kinetic energy operator for isotropic tunnelings ($\Delta_t = 0$) is

$$\hat{H}^0_{\text{hop}} = -\frac{1}{2}t\sum_{j=1}^{M_y}\sum_{l=1}^{M_x}\left(\hat{c}^\dagger_{j,l+1}\hat{c}_{j,l} + \text{h.c}\right) - \frac{1}{2}t\sum_{j=1}^{M_y}\sum_{l=1}^{M_x}\left(\hat{c}^\dagger_{j+1,l}\hat{c}_{j,l} + \text{h.c.}\right)$$

We consider a displacement vector $\vec{u}_{j,l} = \left(u^x_{j,l}, u^y_{j,l}\right)^{\text{T}}$ on every electron lattice site $(j,l)$, following [1–4]. For the undistorted lattice, $u^x_{j,l} = u^y_{j,l} = 0$, whereas distortions are described by $u^x_{j,l} \neq 0, u^y_{j,l} \neq 0$. To proceed, we assume distortion modulated tunneling rates, i.e. (a) for small displacements, the tunneling rates depend linearly on the displacement field, as was, for example, demonstrated to be the case for the prototypical soft semiconductor $\text{MAPbI}_3$ in [5], and (b) that the equilibrium lattice geometry is isotropic and thus the potential energy, $V(\vec{u}_{j,l})$, should exhibit a minimum at $\vec{u}_{j,l} = \vec{0}$. This leads to the following expansion for the rotor-independent Hamiltonian,

$$\begin{aligned}\hat{H}^0_{\text{hop}} \rightarrow \hat{H}'_{\text{hop}} = \hat{H}^0_{\text{hop}} + \hat{V} = &-\frac{1}{2}t\sum_{j=1}^{M_y}\sum_{l=1}^{M_x}\left[1 + \beta\left(u^x_{j,l+1} - u^x_{j,l}\right) + \mathcal{O}\left(\left(u^x_{j+1,l} - u^x_{j,l}\right)^2\right)\right]\left(\hat{c}^\dagger_{j,l+1}\hat{c}_{j,l} + \text{h.c}\right)\\ &-\frac{1}{2}t\sum_{j=1}^{M_y}\sum_{l=1}^{M_x}\left[1 + \beta\left(u^y_{j+1,l} - u^y_{j,l}\right) + \mathcal{O}\left(\left(u^y_{j+1,l} - u^y_{j,l}\right)^2\right)\right]\left(\hat{c}^\dagger_{j+1,l}\hat{c}_{j,l} + \text{h.c.}\right) \qquad (1)\\ &+\frac{K}{2M_xM_y}\sum_{j=1}^{M_y}\sum_{l=1}^{M_x}\left[\left(u^x_{j,l+1} - u^x_{j,l}\right)^2 + \left(u^y_{j+1,l} - u^y_{j,l}\right)^2\right] + \mathcal{O}\left(\left|\vec{u}_{j+1,l} - \vec{u}_{j,l}\right|^3\right),\end{aligned}$$

where $\beta$ is a parameter for the electron-phonon coupling and $K$ is the elastic constant of the lattice. This type of electron-phonon coupling is similar to the Peierls/Su-Schrieffer-Heeger models [6–8]. In scenarios where the lattice distortions $u^{\mu}_{j,l}$ are asymmetric and linear over at least as many unit cells as the polaron state extends, a situation expected to be common for soft semiconductors with characteristic long-wavelength phonon modes [9, 10], we can define

$$\beta\left(u^x_{j,l+1}-u^x_{j,l}\right)\equiv\Delta_t,\quad \beta\left(u^y_{j+1,l}-u^y_{j,l}\right)\equiv-\Delta_t, \tag{2}$$

which gives

$$\hat{H}'_{\text{hop}}=-\frac{1}{2}t\left(1+\Delta_t\right)\sum_{j=1}^{M_y}\sum_{l=1}^{M_x}\left(\hat{c}^\dagger_{j,l+1}\hat{c}_{j,l}+\text{h.c}\right)-\frac{1}{2}t\left(1-\Delta_t\right)\sum_{j=1}^{M_y}\sum_{l=1}^{M_x}\left(\hat{c}^\dagger_{j+1,l}\hat{c}_{j,l}+\text{h.c.}\right)+K\frac{\Delta_t^2}{\beta^2}. \tag{3}$$

Now we can define $t_x=0.5t\left(1+\Delta_t\right)$ and $t_y=0.5t\left(1-\Delta_t\right)$, which gives the expansion of the electron kinetic energy Hamiltonian, as used in the main text, up to second order in $\Delta_t$, $\hat{H}'_{\text{hop}}=\hat{H}^0_{\text{hop}}+\frac{K}{\beta^2}\Delta_t^2$. Hence, the ground state energy of $\hat{H}'_{\text{hop}}+\hat{V}$ is quadratic in the asymmetry parameter $\Delta_t$. The energy minimum of $\hat{H}'_{\text{hop}}$ occurs at $\Delta_t=0$ as per assumption and thus there are no structural distortions in the ground state. However, as demonstrated in the main text, the rotor-electron coupling results in polaron formation depending on $t$, $\Delta_t$, and $V_0$. For fixed $V_0$ and $t$, this additional energy contribution scales quadratically with $\Delta_t$, see Fig. 4(a) in the main text and Fig. 1 below. Therefore, the total effective Hamiltonian reads

$$\hat{H}_{\text{eff}}=\hat{H}^0_{\text{hop}}+\frac{K}{\beta^2}\Delta_t^2-\kappa_{\text{crit}}\Delta_t^2. \tag{4}$$

This term changes the stability properties of the system. For rigid lattices $K>\beta^2\kappa_{\text{crit}}$, the system is stable as the emergence of an anisotropy $\Delta_t=0$ is energetically penalized. However, in the case of soft lattices $K<\beta^2\kappa_{\text{crit}}$, the anisotropy is energetically preferable because the energetic benefit from polaron formation counteracts the effect of lattice rigidity. Thus quantum fluctuations of the coupled rotor-electron-soft lattice system will destabilize the symmetric configuration, $\Delta_t=0$, leading to an asymmetric state, $\Delta_t\neq 0$. Notice that the critical lattice stiffness, as captured by $\kappa_{\text{crit}}\beta^2$, is governed by the ratio of electron-phonon coupling and elastic lattice constant, see Fig. 4(b) in the main text.

*Results.* Consequently, the structural instability caused by the rotor-electron coupling is most pronounced in soft lattices with strong electron-phonon couplings or small elastic lattice constants, i.e. $\beta\ll K$. The $V_0$ dependence of this structural instability is shown in Fig. 1. The critical lattice stiffness $\kappa_{\text{crit}}$ increases until $V_0/t\sim 0.5$, and decreases again for larger $V_0$, see also Fig. 4(b) in the main text, where we depict the corresponding stability-instability phase diagram.

*Jahn-Teller Symmetry-Breaking.* Moreover, from Fig. 1 and Fig. 4(a) in the main text, we can appraise the two-step mechanism as a consequence of the Jahn-Teller theorem [11]. The $\text{FDW}_\mu$ are degenerate within the vGH ansatz for $\Delta_t=0$, but the degeneracy can be lifted, as long as $\Delta_t\neq 0$. Therefore, according to the Jahn-Teller theorem, external fluctuations that couple to a $C_4$ to $C_2$ symmetry-breaking mode, will render the system unstable and force it to a state with $\Delta_t\neq 0$. In the localized ansatz, however, the $\text{FDW}_\mu$ degeneracy is lifted by correctly accounting for the coupling between electrons and rotors. Consequently, there is a minimum fluctuation cutoff that would lead to the $C_4$ to $C_2$ symmetry reduction, i.e. the system exhibits the pseudo-Jahn-Teller effect.

We note that short-wavelength tunneling modulating phonon modes will also lead to a stability-instability relation. However, this analysis is beyond the scope of the present work, and will be presented in a separate follow-up manuscript.

## III. DIRAC-FRENKEL VARIATIONAL PRINCIPLE

We employ the Dirac-Frenkel variational principle [12–14] to determine the ground state energies and wavefunctions within our localized and polaron ansatz. The general form of both variational ansätze $|\psi\rangle$, with single-rotor wavefunctions $\varphi_{i,j}\left(\phi,t\right)$ and electron amplitudes $A_{j,l}\left(t\right)$, reads

$$|\psi\rangle=\sum_{k=1}^{M_y}\sum_{j=1}^{M_x}\prod_{k'=1}^{M_y}\prod_{j'=1}^{M_x}\varphi_{I_y(k,k')I_x(j,j')}\left(\phi_{k',j'}\right)A_{k,j}\left(t\right)\hat{c}^\dagger_{k,j}|0\rangle_{\text{e}}. \tag{5}$$

The choice of index functions $I_\mu(k,k')$ and $A_{k,j}(t)$ determine the physical meaning of the respective variational ansatz. For this general ansatz, the Dirac-Frenkel energy functional is

$$E[|\psi\rangle] = \langle\psi|\hat{H}|\psi\rangle - i\hbar\langle\psi|\frac{\partial}{\partial t}|\psi\rangle + \sum_{i=1}^{M_y}\sum_{j=1}^{M_x}\lambda_{i,j}\left(1-\int \mathrm{d}\phi\,|\varphi_{i,j}(\phi)|^2\right) - \lambda_e\left(\sum_{j=1}^{M_y}\sum_{l=1}^{M_x}|A_{j,l}(t)|^2-1\right), \tag{6}$$

where the Lagrange parameters $\lambda_{i,j}$ and $\lambda_e$ enforce single-rotor and electron normalization. In analogy to the principle of least action, we determine the saddle point of this functional, $\delta E/\delta\varphi^*_{i,j}=0$ and $\delta E/\delta A^*_{i,j}=0$. This gives rise to the respective equations of motion for $\varphi_{j,l}(t)$ and $A_{j,l}(t)$ that we solve by imaginary propagation, i.e. we perform a Wick rotation $t\to -it$, which formally transforms Eq. (26) into a diffusion equation. In the limit $t\to\infty$, all excited states are damped and we converge to the ground state accessible within the respective variational formalism.

## IV. VARIATIONAL LOCALIZED ANSATZ

*Variational State.* This ansatz mimics the localization behavior of the electron wavefunction in the random dipolar field provided by semiclassical rotors in the limit $B \ll t, V_0$. The variational wavefunction for the system being localized on the site $(1,1)$ (without loss of generality), reads

$$|\psi_{1,1}(\phi_{1,1},\ldots,\phi_{M_x,M_y};t)\rangle = \left[\prod_{j=1}^{M_y}\prod_{l=1}^{M_x}\varphi_{j,l}(\phi_{j,l};t)\right]\sum_{j=1}^{M_y}\sum_{l=1}^{M_x}A_{j,l}(t)\hat{c}^\dagger_{j,l}|0\rangle_e. \tag{7}$$

*Equations of Motion.* According to Eq. (6), we derive the Dirac-Frenkel energy functional, $E[\psi_{1,1}]\equiv E[\{\varphi_{j,l}(\phi;t),A_{j,l}(t)\}]$. Subsequently, by invoking the principle of least action, we obtain the equations of motion for the single-rotor wavefunctions,

$$\begin{aligned} i\hbar\frac{\partial}{\partial t}\varphi_{j,l}(\phi;t) = &-B\frac{\partial^2}{\partial\phi^2}\varphi_{j,l}(\phi;t) - \lambda_{j,l}\varphi_{j,l}(\phi;t) + V_0\Big[|A_{j+1,l}(t)|^2\cos\left(\phi-\frac{\pi}{4}\right) + |A_{j+1,l+1}(t)|^2\cos\left(\phi-\frac{3\pi}{4}\right) \\ &+ |A_{j,l}(t)|^2\cos\left(\phi+\frac{\pi}{4}\right) + |A_{j,l+1}(t)|^2\cos\left(\phi+\frac{3\pi}{4}\right)\Big]\varphi_{j,l}(\phi;t), \end{aligned} \tag{8}$$

and the electron occupation amplitudes,

$$\begin{aligned} i\hbar\frac{\partial}{\partial t}A_{j,l}(t) = &-t_x\left(A_{j,l-1}(t)+A_{j,l+1}(t)\right) - t_y\left(A_{j-1,l}(t)+A_{j+1,l}(t)\right) - \lambda_e A_{j,l}(t) \\ &+ V_0\Big[\left(\int \mathrm{d}\phi\ \cos\left(\phi-\frac{\pi}{4}\right)|\varphi_{j-1,l}(\phi;t)|^2\right) + \left(\int \mathrm{d}\phi\ \cos\left(\phi-\frac{3\pi}{4}\right)|\varphi_{j-1,l-1}(\phi;t)|^2\right) \\ &+ \left(\int \mathrm{d}\phi\ \cos\left(\phi+\frac{\pi}{4}\right)|\varphi_{j,l}(\phi;t)|^2\right) + \left(\int \mathrm{d}\phi\ \cos\left(\phi+\frac{3\pi}{4}\right)|\varphi_{j,l-1}(\phi;t)|^2\right)\Big]A_{j,l}(t). \end{aligned} \tag{9}$$

Imaginary time propagation of Eq. (8) and (9) gives the variational ground state energy and wavefunction for the localized ansatz.

*Translated Basis.* As the translation operators are still symmetries of the system, we can evaluate the corresponding polaron states by applying them to $|\psi_{1,1}\rangle$,

$$\hat{\mathcal{T}}_y^m\hat{\mathcal{T}}_x^n|\psi_{1,1}\rangle = \left[\prod_{j=1}^{M_y}\prod_{l=1}^{M_x}\varphi_{j,l}(\phi_{j+m,l+n};t)\right]\sum_{j=1}^{M_y}\sum_{l=1}^{M_x}A_{j,l}(t)\hat{c}^\dagger_{j+m,l+n}|0\rangle_e \tag{10}$$

The translation operators are unitary,

$$\begin{aligned} \hat{\mathcal{T}}_\mu^\dagger\hat{\mathcal{T}}_\mu &= 1 \\ (\hat{\mathcal{T}}_\mu^n)^\dagger\hat{\mathcal{T}}_\mu^k &= \begin{cases}\hat{\mathcal{T}}_\mu^{k-n} & \text{if } k>n\\ (\hat{\mathcal{T}}_\mu^{n-k})^\dagger & \text{if } k<n\end{cases} \end{aligned} \tag{11}$$

and they commute with all the terms of the Hamiltonian. The translated basis is then given by the states $|\psi_{m,n}\rangle = \hat{T}_x^{n-1}\hat{T}_y^{m-1}|\psi_{1,1}\rangle$. The Hamiltonian and overlap matrix in this basis are $H^{\text{loc}}_{m,n,m',n'} = \langle\psi_{1,1}|(\hat{\mathcal{T}}_x^m)^\dagger(\hat{\mathcal{T}}_y^n)^\dagger\hat{H}\hat{\mathcal{T}}_x^{m'}\hat{\mathcal{T}}_y^{n'}|\psi_{1,1}\rangle$ and $S^{\text{loc}}_{m,n,m',n'} = \langle\psi_{1,1}|(\hat{\mathcal{T}}_x^m)^\dagger(\hat{\mathcal{T}}_y^n)^\dagger\hat{\mathcal{T}}_x^{m'}\hat{\mathcal{T}}_y^{n'}|\psi_{1,1}\rangle$, respectively. Solving the generalized eigenvalue problem $\hat{H}^{\text{loc}}|\Psi\rangle = E_{\text{loc}}\hat{S}^{\text{loc}}|\Psi\rangle$ gives the respective polaron states and energies, $|\Psi\rangle = \sum_{m,n} C_{m,n}|\psi_{m,n}\rangle$ and $E_{\text{loc}}$, which are reported in the main text.

## V. PSEUDO LANG-FIRSOV TRANSFORMATION IN THE STRONG COUPLING REGIME

For the validation of the localized ansatz, we perform a pseudo-Lang-Firsov transformation [15, 16] in the strong-coupling limit. Here, we show that the energies of the localized ansatz converge to the energies provided by this transformation in the strong rotor-electron coupling limit.

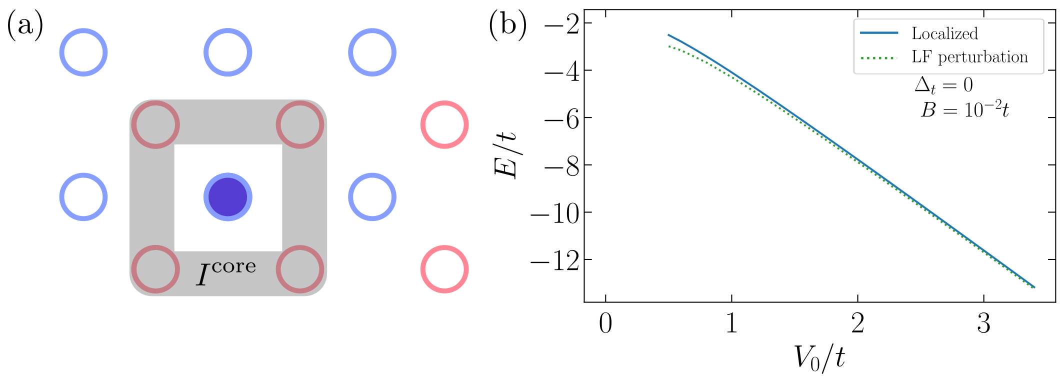


FIG. 2. (a) Sketch of the core rotors, $I^{\text{core}}$ (dark shaded red circles) in the vicinity of the electron site (filled blue circle), relevant for the calculation of the energy correction of Eq. (20). (b) Comparison of the localized ansatz ground state energies with the pseudo Lang-Firsov transformation within second-order perturbation theory.

*Transformation Details.* In the strong coupling limit, $V_0 \gg B, t$, the Hamiltonian is diagonal

$$H_{V_0\to\infty} = \sum_{i,j}\sum_{k}\epsilon_k|i,j\rangle\langle i,j|\otimes|\psi_{(i,j),k}\rangle\langle\psi_{(i,j),k}|, \tag{12}$$

where $\epsilon_k$ and $|\psi_{(i,j),k}\rangle$ are the eigenergies and eigenstates of the rotor system, whose many-body configuration is determined by the multi-index $k$. The state $|i,j\rangle$ denotes the localized eigenstate of the electron on the electron lattice site $(i,j)$. The four rotors surrounding the electron, i.e. $(m,n)\in I^{\text{core}}_{(i,j)} = \{(1,1),(1,M_x),(M_y,1),(M_y,M_x)\}$ as illustrated in Fig. 2(a), obey the Mathieu equation and are hence described by the Mathieu characteristic numbers $n^k_{(m,n)} = 0,1,\dots$ [17]. All other rotors, i.e. $(m,n)\notin I^{\text{core}}_{(i,j)}$ can be described by their respective angular momentum quantum number $l = 0,\pm1,\pm2,\dots$. For details on these definitions, see [18]. The Mathieu and angular momentum quantum numbers uniquely define a many-body rotor wavefunction,

$$|\psi_{(i,j),k}\rangle = \left(\prod_{(m,n)\notin I^{\text{core}}_{(i,j)}}|\psi^{\text{AM}}_{l^k_{(m,n)}}\rangle\right)\prod_{(r,s)\in I^{\text{core}}_{(i,j)}}|\psi^{\text{M}}_{n^k_{(r,s)}}\rangle, \tag{13}$$

where the quantum numbers are specified by the multi-index $k = \left(n^k_{(1,1)}, n^k_{(1,M_y)},\dots,l^k_{(1,2)},l^k_{(1,3)},\dots\right)$. The corresponding energy of a rotor configuration is given by

$$\epsilon_k = \frac{B}{4}\sum_{(m,n)\in I^{\text{core}}_{(i,j)}} f_{n^k_{(m,n)}}\left(\frac{2V_0}{B}\right) + B\sum_{(m,n)\notin I^{\text{core}}_{(i,j)}}\left(l^k_{(m,n)}\right)^2, \tag{14}$$

where $f_{n^k_{(m,n)}}$ is the Mathieu function for Mathieu number $n^k_{(m,n)}$. In the basis generated by $|\psi_{(i,j),k}\rangle$, we can write

the full Hamiltonian as

$$
\begin{aligned}
H = &- t_x \sum_{i,j} \sum_{k,l} \Big( \langle \psi_{(i,j),k} | \psi_{(i,j+1),l} \rangle |i,j\rangle\langle i,j+1| \otimes |\psi_{(i,j),k}\rangle\langle\psi_{(i,j+1),l}| + \text{h.c.} \Big) \\
&- t_y \sum_{i,j} \sum_{k,l} \Big( \langle \psi_{(i,j),k} | \psi_{(i+1,j),l} \rangle |i,j\rangle\langle i+1,j| \otimes |\psi_{(i,j),k}\rangle\langle\psi_{(i+1,j),l}| + \text{h.c.} \Big) \\
&+ \sum_{i,j} \sum_{k} \epsilon_k |i,j\rangle\langle i,j| \otimes |\psi_{(i,j),k}\rangle\langle\psi_{(i,j),k}|.
\end{aligned} \tag{15}
$$

Employing the translation invariance in both $x$ and $y$ directions, we can block-diagonalize the electron part in momentum space with the basis transformation $|q_x, q_y\rangle = \frac{1}{\sqrt{M_x M_y}} \sum_{i,j,} e^{i\frac{2\pi q_y}{M_y} i} e^{i\frac{2\pi q_x}{M_x} j} |i,j\rangle$, which gives $\hat{H} = \sum_{q_y,q_x} H_{q_y,q_x} \otimes |q_y, q_x\rangle\langle q_y, q_x|$, where $H_{q_y,q_x} = H^0_{q_y,q_x} + H^{\text{kin}}_{q_y,q_x}$. The localization of the electron is described by the diagonal Hamiltonian $H^0_{q_y,q_x} = \sum_k \epsilon_k |\psi_k\rangle\langle\psi_k|$, and the electron kinetic energy that carries the localized states on the lattice is given by

$$
H^{\text{kin}}_{q_y,q_x} = -t_x \sum_{k,l} \Big( O^{\text{R}}_{k,l} e^{i\frac{2\pi}{M_x} q_x} |\psi_k\rangle\langle\psi_l| + \text{h.c.} \Big) - t_y \sum_{k,l} \Big( O^{\text{D}}_{k,l} e^{i\frac{2\pi}{M_y} q_y} |\psi_k\rangle\langle\psi_l| + \text{h.c.} \Big) \tag{16}
$$

Here, we defined the overlap elements $O^{\text{R}}_{k,l}$ and $O^{\text{D}}_{k,l}$ that couple the rotors along the respective lattice directions,

$$
\begin{aligned}
O^{\text{R}}_{k,l} = &\Bigg[ \prod_{(m,n)\neq I^{\text{core,ext}}} \langle \psi^{\text{AM}}_{l^k_{(m,n)}} | \psi^{\text{AM}}_{l^l_{(m,n-1)}} \rangle \Bigg] \times \langle \psi^{\text{M}}_{n^k_{(M_y,M_x)}} | \psi^{\text{AM}}_{l^l_{(M_y,M_x-1)}} \rangle \times \langle \psi^{\text{M}}_{n^k_{(M_y,1)}} | \psi^{\text{M}}_{n^l_{(M_y,M_x)}} \rangle \\
&\times \langle \psi^{\text{AM}}_{l^k_{(M_y,2)}} | \psi^{\text{M}}_{n^l_{(M_y,1)}} \rangle \times \langle \psi^{\text{M}}_{n^k_{(1,M_x)}} | \psi^{\text{AM}}_{l^l_{(1,M_x-1)}} \rangle \times \langle \psi^{\text{M}}_{n^k_{(1,1)}} | \psi^{\text{M}}_{n^l_{(1,M_x)}} \rangle \times \langle \psi^{\text{AM}}_{l^k_{(1,2)}} | \psi^{\text{M}}_{n^l_{(1,1)}} \rangle
\end{aligned} \tag{17}
$$

and

$$
\begin{aligned}
O^{\text{D}}_{k,l} = &\Bigg[ \prod_{(m,n)\neq I^{\text{core,ext}}} \langle \psi^{\text{AM}}_{l^k_{(m,n)}} | \psi^{\text{AM}}_{l^l_{(m-1,n)}} \rangle \Bigg] \times \langle \psi^{\text{M}}_{n^k_{(M_y,M_x)}} | \psi^{\text{AM}}_{l^l_{(M_y-1,M_x)}} \rangle \times \langle \psi^{\text{M}}_{n^k_{(1,M_x)}} | \psi^{\text{M}}_{n^l_{(M_y,M_x)}} \rangle \\
&\times \langle \psi^{\text{AM}}_{l^k_{(2,M_x)}} | \psi^{\text{M}}_{n^l_{(1,M_x)}} \rangle \times \langle \psi^{\text{M}}_{n^k_{(M_y,1)}} | \psi^{\text{AM}}_{l^l_{(M_y-1,1)}} \rangle \times \langle \psi^{\text{M}}_{n^k_{(1,1)}} | \psi^{\text{M}}_{n^l_{(M_y,1)}} \rangle \times \langle \psi^{\text{AM}}_{l^k_{(2,1)}} | \psi^{\text{M}}_{n^l_{(1,1)}} \rangle.
\end{aligned} \tag{18}
$$

To obtain the correction to the ground state energy of a localized state, we perform second-order perturbation theory in the tunneling $t$. The ground state of the localized Hamiltonian $H^0_{q_y,q_x}$ is given by $k = 0$, i.e. $H^0_{q_y,q_x}|\psi^{(0)}_0\rangle = \epsilon^{(0)}_0|\psi^{(0)}_0\rangle$. The first order correction is

$$
\epsilon^{(1)}_0 = \langle \psi^{(0)}_0 | H_{\text{int}} | \psi^{(0)}_0 \rangle = -t_x \Big( O^{\text{R}}_{0,0} e^{i\frac{2\pi}{M_x} q_x} + \text{c.c.} \Big) - t_y \Big( O^{\text{D}}_{0,0} e^{i\frac{2\pi}{M_y} q_y} + \text{c.c.} \Big) \tag{19}
$$

and the second order correction is

$$
\epsilon^{(2)}_0 = \sum_{n\neq 0} \frac{\Big| \langle \psi^{(0)}_0 | H_{\text{int}} | \psi^{(0)}_n \rangle \Big|^2}{\epsilon^{(0)}_0 - \epsilon^{(0)}_n} = 2\left(t_x^2 + t_y^2\right) \sum_{n\notin I^{\text{core}}} \frac{|\tilde{O}^{\text{L}}_{0,n}|^2}{\epsilon^{(0)}_0 - \epsilon^{(0)}_n} + \sum_{n\in I^{\text{core}}} \frac{\Big| -t_x \Big( \tilde{O}^{\text{R}}_{0,n} + \tilde{O}^{\text{L}}_{0,n} \Big) - t_y \Big( \tilde{O}^{\text{U}}_{0,n} + \tilde{O}^{\text{D}}_{0,n} \Big) \Big|^2}{\epsilon^{(0)}_0 - \epsilon^{(0)}_n}. \tag{20}
$$

*Energy Comparison.* In Fig. 2(b), we compare the energies of the localized ansatz with the ones obtained from the second-order pseudo-Lang-Firsov transformation. We show that they indeed converge in the strong coupling limit.

## VI. CLASSICAL TREATMENT OF THE ROTORS

This section summarizes our approach to obtain the classical ground state of the system in the limit $B \to 0$, which provides a valuable sanity check of our calculations. Our approach is based on the gradient descent minimization method.

*Classical Rotor Limit.* In the classical limit $\hbar \to 0 \Leftrightarrow B \to 0$, the rotational energy of the lattice vanishes in any equilibrium state, $\hat{H}_{\text{rot}} = 0$. This in turn implies that the orientations of the rotors are merely parameters of the

resulting Hamiltonian $\hat{H}_{\rm C}(\phi_{1,1},\ldots,\phi_{M_y,M_x}) = \hat{H}_{\rm hop} + \hat{H}_{\rm int}(\phi_{1,1},\ldots,\phi_{M_y,M_x})$, which affect the potential experienced by the electron *via* $\hat{H}_{\rm int}$, see Eq. (4). For ease of notation herewith we define a given rotor configuration as the set of particular orientations *via* $\{\phi^{(k)}\} = \{\phi^{(k)}_{1,1},\ldots,\phi^{(k)}_{M_y,M_x}\}$, where $k$ is an index parametrizing the particular configuration that will be omitted when we refer to all possible sets. The ground state energy of $\hat{H}_{\rm C}(\{\phi\})$, $E_{\rm G}(\{\phi\})$, can be calculated by elementary techniques for any configuration of $\{\phi\}$, as it corresponds to a single electron hopping in a square lattice with varying on-site potentials. Therefore, evaluating the classical ground state equates to finding the configuration $\{\phi^{(G)}\}$ that results in the minimal $E_{\rm G}(\{\phi^{(G)}\})$. However, since there are $M = M_xM_y$ rotors, the optimization problem remains highly multidimensional.

*Gradient Descent.* Despite that the full functional form of $E_{\rm G}(\{\phi\})$ is not available, the fact that it corresponds to the ground state energy of a quantum system, allows us to efficiently calculate the derivative of the electron energy at any particular rotor configuration $\{\phi\}\}$. Indeed, given a configuration $\{\phi^{(0)}\}$, we can diagonalize $\hat{H}_{\rm C}(\{\phi^{(0)}\})$, obtaining the ground state eigenenergy $E_{\rm G}(\{\phi^{(0)}\})$ and eigenstate $|\psi_{\rm G}(\{\phi^{(0)}\})\rangle$ and then the derivative over any $\phi_{j,l}$ rotor coordinate can be calculated *via* the Feynman-Hellman theorem

$$\left.\frac{\partial E_{\rm G}}{\partial \phi_{j',l'}}\right|_{\{\phi^{(0)}\}} = \left\langle \psi_{\rm G}(\{\phi^{(0)}\}) \middle| \frac{\partial \hat{H}_{\rm C}}{\partial \phi_{j',l'}} \middle| \psi_{\rm G}(\{\phi^{(0)}\}) \right\rangle. \tag{21}$$

Notice that the derivative of the classical Hamiltonian is of a simple form,

$$\begin{aligned}\frac{\partial \hat{H}_{\rm C}}{\partial \phi_{j',l'}} = V_0\Big[&\hat{c}^\dagger_{j'+1,l'}\hat{c}_{j'+1,l'}\sin\left(\phi_{j',l'} - \frac{\pi}{4}\right) + \hat{c}^\dagger_{j',l'}\hat{c}_{j',l'}\sin\left(\phi_{j',l'} + \frac{\pi}{4}\right) \\ &+ \hat{c}^\dagger_{j'+1,l'+1}\hat{c}_{j'+1,l'+1}\sin\left(\phi_{j',l'} - \frac{3\pi}{4}\right) + \hat{c}^\dagger_{j',l'+1}\hat{c}_{j',l'+1}\sin\left(\phi_{j',l'} + \frac{3\pi}{4}\right)\Big],\end{aligned} \tag{22}$$

making this calculation computationally very efficient. Having the gradient for all rotors, we can implement a gradient descent approach based on the iteration

$$\phi^{(i+1)}_{j,l} = \phi^{(i)}_{j,l} - \alpha \left.\frac{\partial E_{\rm G}}{\partial \phi_{j,l}}\right|_{\{\phi^{(i)}\}}, \tag{23}$$

where $\alpha$ is a control parameter determining how fast the rotor angles change with each iteration. However, this parameter can be understood in a physical picture, which allows us to heavily optimize our calculations.

Let us consider that the rotors evolve classically but are strongly damped by some external friction source, such that their moment of inertia can be dropped, i.e. they are within the overdamped regime. Then the equation of motion for the system would read $\dot{\phi}_{j,l}(t) = \frac{1}{\gamma}F_{j,l}(t)$, where $\gamma$ is the friction constant and the force is given by $F_{j,l}(t) = -\frac{\partial E_{\rm G}}{\partial \phi_{j,l}}\big|_{\{\phi(t)\}}$. It is easy to see that if we try to time-integrate this problem within the Euler method, then Eq. (23) describes the iterative sequence that gives $\phi_{j,l}(t_0 + i\delta t) = \phi^{(i)}_{j,l}$ from the initial state $\phi_{j,l}(t_0) = \phi^{(0)}_{j,l}$. Here $\alpha = \delta t/\gamma$, where $\delta t > 0$ is the time-step. It might not be obvious at first glance, but mapping Eq. (23) to the solution of a time-dependent friction problem by the Euler method leads to a deep understanding on how our methodology converges. First notice that the force stemming from Eq. (22) can always be written as $F_{j,l}(t) = V_0\kappa_{j,l}(t)\sin(\phi_{j,l} - \phi^{\rm pop}_{j,l}(t))$, where $\kappa_{j,l}(t) < 1$, $\phi^{\rm pop}_{j,l}(t)$ are simple functions of the populations of the neighboring sites $n_{j,l}(t)$. These expressions read

$$\begin{aligned} n_{j,l}(t) =& \langle\psi_{\rm G}(\{\phi(t)\})|\hat{c}^\dagger_{j,l}\hat{c}_{j,l}|\psi_{\rm G}(\{\phi(t)\})\rangle, \\ \kappa_{j,l}(t) =& \sqrt{[n_{j,l}(t) - n_{j+1,l+1}(t)]^2 + [n_{j+1,l}(t) - n_{j,l+1}(t)]^2}, \\ \phi^{\rm pop}_{j,l}(t) =& {\rm sign}\left([n_{j+1,l}(t) + n_{j+1,l+1}(t)] - [n_{j,l}(t) + n_{j+1,l+1}(t)]\right) \\ &\times \arccos\left(\frac{[n_{j+1,l}(t) + n_{j,l}(t)] - [n_{j+1,l+1}(t) + n_{j,l+1}(t)]}{\sqrt{2}\kappa_{j,l}(t)}\right)\end{aligned} \tag{24}$$

Obviously, $F_{j,l}(t)$ is a function with a single minimum and maximum for each rotor at every point in time $t$, and thus no multi-stability is expected at the single rotor level. Therefore, for a given initial state, the system will deterministically converge to a unique configuration that minimizes the energy of all rotors, i.e. there is a single attractor. Of course, $\hat{H}_{\rm C}(\{\phi\})$ is translationally invariant in the sense that it should reproduce the same ground state

energy if all the rotors are shifted via the transformation $\phi^{(S)}_{j,l} = \phi^{(O)}_{(j+j_s) \bmod M_y,(l+l_s) \bmod M_x}$. This creates a strong initial state dependence, which we exploit to identify the analytic continuation of the exact solution for $V_0 \to \infty$ and for the electron localized in the site $j = l = 1$, in the case of finite $V_0$ by setting the former as our initial condition. This solution reads

$$\phi^{(0)}_{j,l} = \begin{cases} \frac{3\pi}{4} & \text{if } j \le \frac{M_y}{2} \text{ and } l \le \frac{M_x}{2}, \\ \frac{\pi}{4} & \text{if } j \le \frac{M_y}{2} \text{ and } l > \frac{M_x}{2}, \\ -\frac{3\pi}{4} & \text{if } j > \frac{M_y}{2} \text{ and } l \le \frac{M_x}{2}, \\ -\frac{\pi}{4} & \text{if } j > \frac{M_y}{2} \text{ and } l > \frac{M_x}{2}. \end{cases} \tag{25}$$

The expectation that the ground states will be adiabatically connected to the $V_0 \to \infty$ solutions stems from the second-order of the transitions among the different regimes observed within the variational localized ansatz.

Notice also that if a rotor is close to its equilibrium state such that $\phi_{j,l} \approx \phi^{\text{pop}}_{j,l}(t) \approx \phi^{\text{pop}}_{j,l}(t \to \infty)$, then the solution will be $\phi_{j,t}(t) = \phi^{\text{pop}}_{j,t}(t \to \infty) + (\phi_{j,t}(t_0) - \phi^{\text{pop}}_{j,t}(t \to \infty)) \exp\left(-\frac{V_0 \kappa}{\gamma} t\right)$ and thus the rotor will converge exponentially fast to its ground state. The fact that in this case the equation of motion is linear also allows us to use the theorems for the stability of the Euler method to pick the optimal value of $\alpha$. It is known that for equations of the form $y'(t) = zy(t)$, where $z$ is a complex constant value, the Euler method is stable only if $|z+1| \le 1$. Applying this to our case, we get $|\frac{V_0 \kappa_{j,l}(t) \delta t}{\gamma} + 1| \le 1$ and thus $V_0 \alpha \kappa_{j,l}(t) < 1$, and since $\kappa_{j,l}(t) \le 1$ for all rotors, it is guaranteed that for $\alpha \lessapprox 1/V_0$, the Euler method will be stable. To produce an accurate trajectory for the time-dependent problem one would want $\alpha$ to be much lower than the threshold of stability but since we are only interested in the final equilibrium state, we can afford using a large $\alpha$ for improved numerical efficiency.

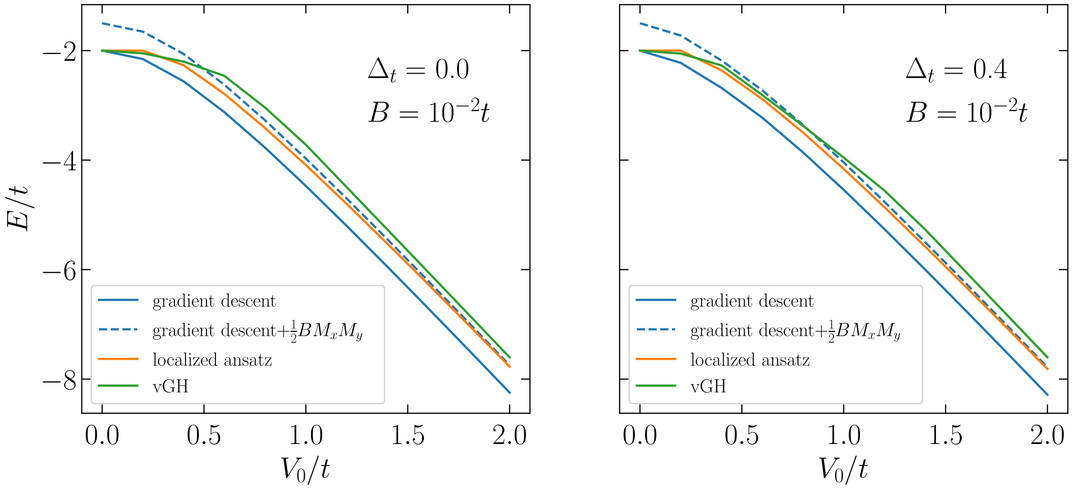


FIG. 3. Comparison of the classical energies with the energies of the localized and the vGH ansatz for two lattice asymmetries, $\Delta_t = 0$ and $\Delta_t = 0.4$. The blue dashed lines correspond to the energies obtained from gradient descent, corrected by the classical rotor self-energy, $BM_xM_y/2$. The gradient descent energies match well with the energies of the localized ansatz in the strong coupling regime.

*Energy Comparison.* We find that the energies obtained with this gradient descent approach underestimate the variational energies, see the solid blue lines in Fig. 3. However, this classical result neglects the rotor kinetic energy for finite $B$. According to the virial theorem, the self-energy of every rotor can be approximated by $B/2$, and thus we correct the gradient descent energy by adding the total self-energy of the rotor system, $BM_xM_y/2$, see the dashed blue lines in Fig. 3. We find that the corrected gradient descent energies agree well with the energies of the localized ansatz in the strong coupling regime. For intermediate couplings, the corrected gradient descent energies lie between the localized and vGH energies. Furthermore, the corrected classical energies reproduce the energy dependence on the tunneling anisotropy $\Delta_t$, see Fig. 1, and the properties of the classical states give rise to a phase diagram that is qualitatively similar to the one from the localized ansatz, see Fig. 5. Therefore, the classical treatment of the rotors validates our findings of the stability-instability transition.

## VII. VARIATIONAL POLARON ANSATZ IN THE CO-MOVING FRAME

*Variational State.* In the weak-coupling limit, the rotor-electron coupling dresses the plane-wave states of the electron and intuitively acts like a drag. To mimic this behavior, we apply a variational Gross-Hartree (vGH) polaron ansatz in the co-moving frame [18, 19],

$$|\psi_{q_x,q_y}\rangle = \sum_{k=1}^{M_y}\sum_{j=1}^{M_x} \frac{e^{i\frac{2\pi q_x}{M_x}j}}{\sqrt{M_x}} \frac{e^{i\frac{2\pi q_y}{M_y}k}}{\sqrt{M_y}} \prod_{k'=1}^{M_y}\prod_{j'=1}^{M_x} \varphi_{I_y(k,k')I_x(j,j')}\left(\phi_{k',j'}\right) \hat{c}^\dagger_{kj}|0\rangle_{\mathrm{e}}.$$

Here, the index functions $I_\mu(k,k') = \mod(M_\mu + k' - k, M_\mu) + 1$ guarantee that the rotor index is always chosen relative to the electron position $(k,j)$.

*Equations of Motion.* We compute the Dirac-Frenkel energy functional according to Eq. (6). From this, by invoking the principle of least action, we get the equations of motion for the single-rotor wavefunctions,

$$\begin{aligned} i\frac{\partial}{\partial t}\varphi_{m,n}(\phi,t) &= -B\frac{\partial^2}{\partial\phi^2}\varphi_{m,n}(\phi,t) - t_x\left(e^{-i\frac{2\pi q_x}{M_x}} \prod_{(e,f)\neq(m,n)} \int \mathrm{d}\phi\, \varphi^*_{e,f}(\phi)\,\varphi_{e,f+1}(\phi)\,\varphi_{m,n+1}(\phi) + \mathrm{c.c.}\right) \\ &- t_y\left(e^{-i\frac{2\pi q_y}{M_y}} \prod_{(e,f)\neq(m,n)} \int \mathrm{d}\phi\, \varphi^*_{e,f}(\phi)\,\varphi_{e+1,f}(\phi)\,\varphi_{m+1,n}(\phi) + \mathrm{c.c.}\right) + V_0\Big(\cos\left(\phi+\eta_{M_y1}\right)\delta_{m,M_y}\delta_{n,1} \\ &+ \cos\left(\phi+\eta_{M_yM_x}\right)\delta_{m,M_y}\delta_{n,M_x} + \cos\left(\phi+\eta_{11}\right)\delta_{m,1}\delta_{n,1} + \cos\left(\phi+\eta_{1M_x}\right)\delta_{m,1}\delta_{n,M_x}\Big)\varphi_{m,n}(\phi,t) - \lambda_{m,n}\varphi_{m,n}(\phi,t)\,. \end{aligned} \tag{26}$$

Imaginary time propagation of Eq. (26), as described in Part III, gives the variational ground state energy and wavefunction of this ansatz. For the vGH phase diagram and a comparison of the vGH energies with the ones of the localized ansatz, see Part IX.

## VIII. PERTURBATION THEORY IN THE WEAK COUPLING REGIME

In this part, we perform a BW perturbation theory calculation [18, 20, 21] and show that the vGH Ansatz agrees with the perturbative treatment in the weak coupling regime. Furthermore, we investigate the energetic behavior of the system in the limiting case of classical rotational constants, $B \to 0$.

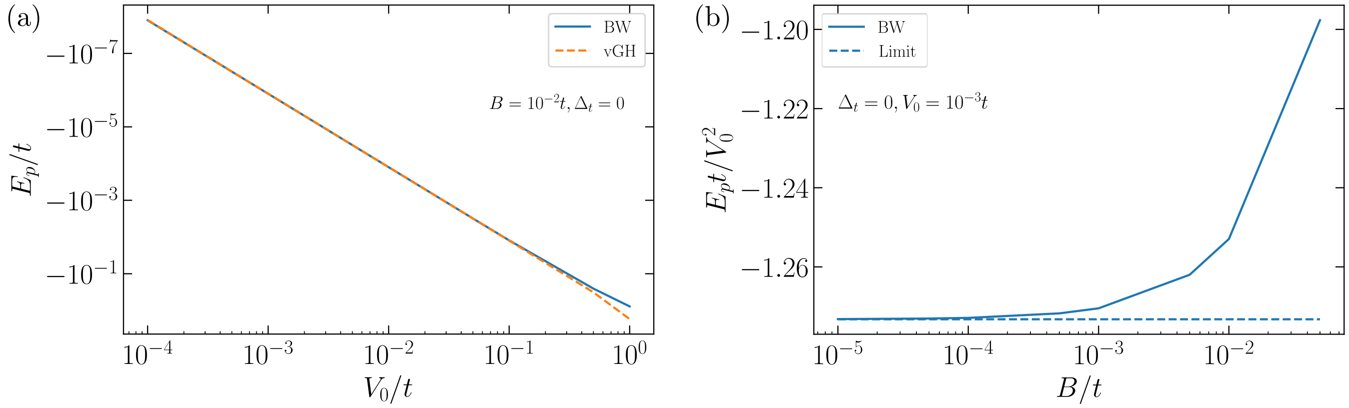


FIG. 4. (a) Comparison of the polaron energy $E_p = E + 2t$ at $\mathbf{k} = 0$ between vGH and BW perturbation theory in the weak coupling regime for $B = 10^{-2}t$. (b) Scaling of the polaron energy with decreasing rotational constant $B \to 0$.

*Perturbation Theory.* In the zero coupling limit, $V_0 = 0$, the rotational and electronic degrees of freedom decouple such that $|\mathbf{m} = \left(m_{1,1}, m_{1,2}, \ldots, m_{M_y,M_x}\right)\rangle$ defines the rotational eigenstates with angular momentum quantum numbers $m_{i,j} = 0, \pm1, \ldots$ for the $i,j$-th rotor and $|\mathbf{k} = (k_x,k_y)\rangle = \frac{1}{\sqrt{M_yM_x}}\sum_{i,j} e^{ik_yi}e^{ik_xj}|i,j\rangle$ defines the electronic eigenstates with quasimomenta $k_{x,y} = 2\pi q_{x,y}/M_{x,y}, q_{x,y} = 0,1,\ldots,M_{x,y}-1$. The energy in terms of these quantum numbers is then given by $E_{\mathbf{k},\mathbf{m}} = \epsilon^{\mathrm{el}}_{\mathbf{k}} + \epsilon^{\mathrm{rot}}_{\mathbf{m}}$, where $\epsilon^{\mathrm{el}}_{\mathbf{k}} = -2t_x\cos(k_x) - 2t_y\cos(k_y)$ and $\epsilon^{\mathrm{rot}}_{\mathbf{m}} = B\sum_{i,j} m^2_{i,j}$. The

perturbation of the exactly solvable zero coupling limit is given by the interaction term $\hat{H}_{\text{int}}$. The interaction acts such that a state $|\mathbf{k},\mathbf{m}\rangle$ just couples to $|\mathbf{k},\mathbf{m}\pm\mathbf{e}_{ij}\rangle$, where $\mathbf{e}_{i,j}$ is a unit vector that raises or lowers the angular momentum quantum number of the $i,j$-th rotor. Hence, within BW perturbation theory, we can expand the perturbative wavefunction as follows

$$|\psi(\mathbf{k},\mathbf{m})\rangle = \alpha_{\mathbf{k},\mathbf{m}}|\mathbf{k},\mathbf{m}\rangle + \sum_{\mathbf{k}'}\sum_{i,j}\Big(\beta_{\mathbf{k};\mathbf{k}';\mathbf{m};i,j}|\mathbf{k}',\mathbf{m}+\mathbf{e}_{i,j}\rangle + \gamma_{\mathbf{k};\mathbf{k}';\mathbf{m};i,j}|\mathbf{k}',\mathbf{m}-\mathbf{e}_{i,j}\rangle\Big). \tag{27}$$

The expansion coefficients $\alpha_{\mathbf{k},\mathbf{m}}, \beta_{\mathbf{k};\mathbf{k}';\mathbf{m};i,j}$ and $\gamma_{\mathbf{k};\mathbf{k}';\mathbf{m};i,j}$ depend on the energy of the system $E$ and are given as

$$\alpha_{\mathbf{k},\mathbf{m}} = \sqrt{Z},\ \beta_{\mathbf{k};\mathbf{k}';\mathbf{m};i,j} = -\sqrt{Z}\frac{\langle\mathbf{k}',\mathbf{m}+\mathbf{e}_{i,j}|\hat{H}_{\text{int}}|\mathbf{k},\mathbf{m}\rangle}{\epsilon^{\text{el}}_{\mathbf{k}'}+\epsilon^{\text{rot}}_{\mathbf{m}+\mathbf{e}_{i,j}}-E} \text{ and } \gamma_{\mathbf{k};\mathbf{k}';\mathbf{m};i,j} = -\sqrt{Z}\frac{\langle\mathbf{k}',\mathbf{m}-\mathbf{e}_{i,j}|\hat{H}_{\text{int}}|\mathbf{k};\mathbf{m}\rangle}{\epsilon^{\text{el}}_{\mathbf{k}'}+\epsilon^{\text{rot}}_{\mathbf{m}-\mathbf{e}_{i,j}}-E} \tag{28}$$

where the polaron residue $Z$ is determined from the normalization condition $\langle\psi(\mathbf{k},\mathbf{m})|\psi(\mathbf{k},\mathbf{m})\rangle = 1$. From $E = \langle\psi(\mathbf{k},\mathbf{m})|\hat{H}|\psi(\mathbf{k},\mathbf{m})\rangle$ we get

$$E = \epsilon^{\text{el}}_{\mathbf{k}} + \epsilon^{\text{rot}}_{\mathbf{m}} - \Sigma_{\mathbf{k},\mathbf{m}}(E)\,. \tag{29}$$

with the energy dependent self energy

$$\Sigma_{\mathbf{k},\mathbf{m}}(E) = \sum_{k'_x,k'_y}\sum_{i,j}\frac{\left|\langle\mathbf{k},\mathbf{m}|\hat{H}_{\text{int}}|\mathbf{k}',\mathbf{m}+\hat{\mathbf{e}}_{ij}\rangle\right|^2}{\epsilon^{\text{tr}}_{\mathbf{k}'}+\epsilon^{\text{rot}}_{\mathbf{m}+\hat{\mathbf{e}}_{ij}}-E} + \frac{\left|\langle\mathbf{k},\mathbf{m}|\hat{H}_{\text{int}}|\mathbf{k}',\mathbf{m}-\hat{\mathbf{e}}_{ij}\rangle\right|^2}{\epsilon^{\text{tr}}_{\mathbf{k}'}+\epsilon^{\text{rot}}_{\mathbf{m}-\hat{\mathbf{e}}_{ij}}-E}. \tag{30}$$

Inserting the expression for the respective matrix elements gives the self-energy

$$\Sigma_{\mathbf{k},0}(E) = \frac{2V_0^2}{M_xM_y}\sum_{k'_x,k'_y}\frac{1-\cos(k_x-k'_x)\cos\left(k_y-k'_y\right)}{B-E-2t_x\cos(k'_x)-2t_y\cos\left(k'_y\right)}, \tag{31}$$

which corrects the ground state configuration where all rotors are in their angular momentum ground state, i.e. $\mathbf{m}=0$. We integrate the expression for the self-energy numerically, as there is no readily available analytic solution and henceforth obtain the energy $E$ iteratively according to Eq. (29). Within this perturbative approach, the polaron energy is defined as $E_p = E - \epsilon^{\text{el}}_{\mathbf{k}} = -\Sigma_{\mathbf{k},0}\left(E_p+\epsilon^{\text{el}}_{\mathbf{k}}\right)$ and hence for a stationary electron $E_p(\mathbf{k}=0) = E+2t$.

*Energy Comparison.* In Fig. 4(a), we compare the BW perturbation energies with the corresponding vGH energies. The BW perturbation theory energies agree with the vGH energies until $V_0 \sim 0.1t$. With increasing $V_0$, the rotor-electron interaction excites a large number of rotors, rendering the perturbative treatment invalid.

*Classical Rotors.* An analysis of the scaling of the self-energy $\Sigma_{\mathbf{k},0}$ reveals that the polaron energy does not diverge in the limit $B\to0$. Mathematically, this can be seen from Eq. (31), because in the limit $B\to0, V_0\to0$, there is no pole for $E\to-2t$ (note that $E<-2t$). We show the asymptotic scaling of $E_p$ in the limit $B\to0$ in Fig. 4(b). This is in contrast to the self-energy in one dimension, i.e. if $t_\mu=0$ while $t_{\nu\neq\mu}=t$ [18]. In one dimension and the limit of classical rotors, $B\to0$, the self-energy diverges, indicating behavior similar to Anderson orthogonality catastrophe. In this limit, an excitation created by an infinitely small, but finite rotor-electron interaction induces an infinitely extended, long-range ferroelectric polarized state. In contrast, in two dimensions, a small but finite interaction leads to an (exponential) localization of the electron in the potential energy landscape provided by the classical rotors. Hence, the classical limit is well-behaved in two dimensions.

## IX. COMPARISON OF THE VARIATIONAL METHODS

In this part, we provide additional data for the comparison of the two variational approaches and the classical gradient descent.

*Phase Diagrams.* First, we compare the phase diagrams emerging within the variational vGH, the localized ansatz, and the classical gradient descent. In the vGH ansatz, in analogy to the localized ansatz, we find four classes of ground states, see the $\Delta_t$–$V_0$ phase diagram in Fig. 5(a). Characteristic of this phase diagram are the sharp phase transitions and the degeneracy of the uncoupled, orthogonal FDW$_\mu$ states at $\Delta_t=0$ for intermediate coupling strengths, which

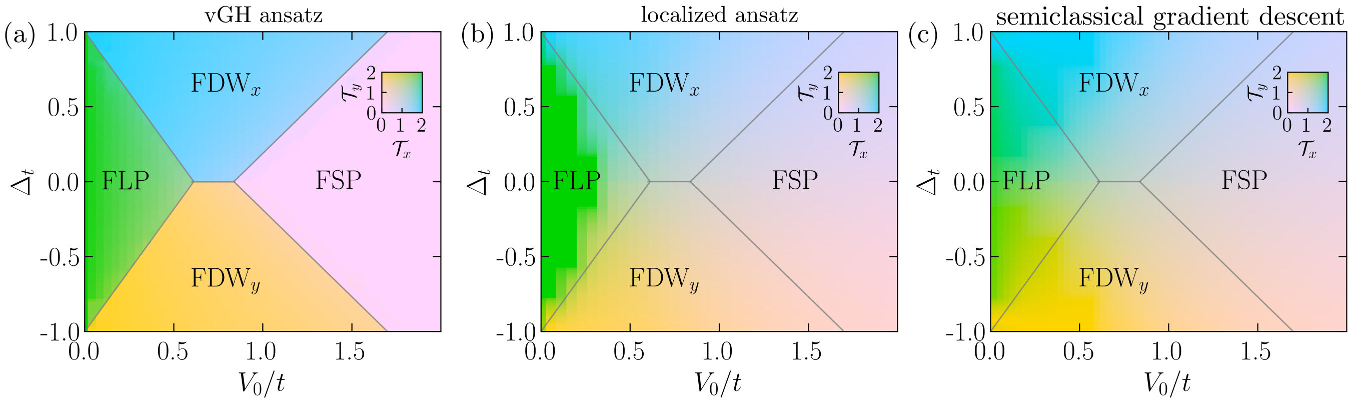


FIG. 5. Comparison of the phase diagrams obtained within the three approaches: (a) vGH ansatz, (b) localized ansatz and (c) classical gradient descent. In (a) and (b), the rotational constant is $B = 10^{-2}t$, while in (c) $B = 0$. The superimposed grey lines in (b) and (c) are drawn to highlight the sharp phase transitions emerging within the vGH ansatz.

is lifted for $\Delta_t \neq 0$. On the other hand, the phase diagram of the localized ansatz shows a smooth crossover from FLP to FDW$_\mu$ and FSP states, see Fig. 5(b). Hence, this ansatz describes the correlations between rotors and the electron more accurately. We note that the phase diagram in Fig. 3(b) of the main text is a combination of Fig. 5(a) and (b), where we take the variational state with the minimum energy for every $(V_0/t, \Delta_t)$ point. The phase diagram obtained from the classical gradient descent calculation is comparable to the one of the localized ansatz, see Fig. 5(c). Notice here that the order parameters $\mathcal{T}_\mu$ do not depend much on $B$, as long as we are in the semiclassical regime $B \ll t$.

*Energy Comparison.* In Fig. 6(a), we show the ground state energy in the $\Delta_t$–$V_0$ plane, always taking the minimum energy between localized and vGH ansatz. In Fig. 6(b), we show the energetic difference between the vGH polaron and the localized ansatz for various $\Delta_t$. For extremely asymmetric lattices, the system is better described by the vGH ansatz, while for weakly asymmmetric lattices, $\Delta_t \sim 0$, the localized ansatz better captures the interplay between localization driven by the rotor-electron coupling and transport of the electron. This indicates that the rotor-electron correlations have to be treated differently in one and two dimensions, also cf. [18].

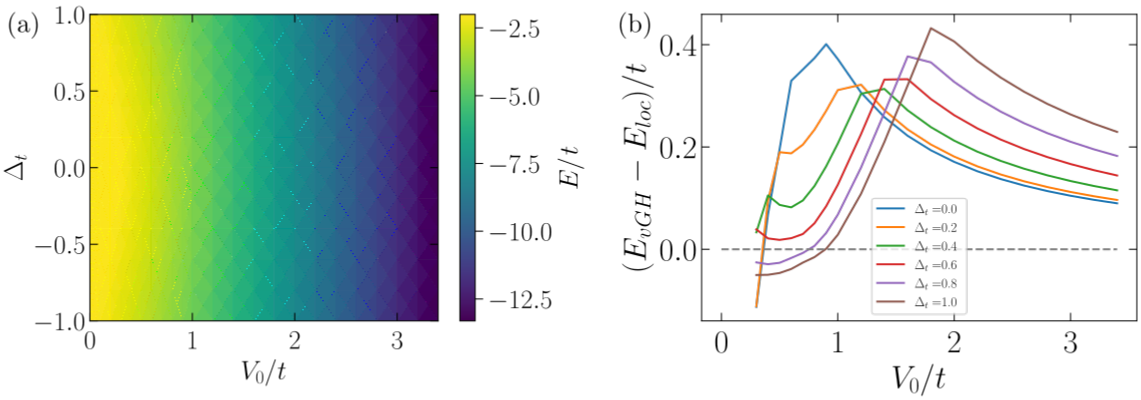


FIG. 6. (a) Variational ground state energy in the $\Delta_t$–$V_0$ plane, always taking the minimum energy between localized and vGH ansatz at every data point. (b) Difference between the vGH and localized ansatz energy for different lattice asymmetries. Below an interaction strength of $V_0 \sim 0.35t$, the validity of the localized ansatz breaks down and hence we do not show the respective data points.


[1] J. Riera and A. Moreo, Phys. Rev. B **73**, 014518 (2006).
[2] C. Alberto Lamas, J. Phys. Soc. Jpn. **78**, 014602 (2009).

[3] V. M. Pereira, A. H. Castro Neto, and N. M. R. Peres, Phys. Rev. B **80**, 045401 (2009).
[4] L. Zhang, Y. Hao, W. Qin, S. Xie, and F. Qu, Phys. Rev. B **102**, 214303 (2020).
[5] M. Z. Mayers, L. Z. Tan, D. A. Egger, A. M. Rappe, and D. R. Reichman, Nano Lett. **18**, 8041 (2018).
[6] C. Zhang, N. V. Prokof'ev, and B. V. Svistunov, Phys. Rev. B **104**, 035143 (2021).
[7] B. Xing, W.-T. Chiu, D. Poletti, R. Scalettar, and G. Batrouni, Phys. Rev. Lett. **126**, 017601 (2021).
[8] N. V. Prokof'ev and B. V. Svistunov, Phys. Rev. B **106**, l041117 (2022).
[9] F. Wang, Y. Fu, M. E. Ziffer, Y. Dai, S. F. Maehrlein, and X.-Y. Zhu, J. Am. Chem. Soc. **143**, 5 (2020).
[10] F. Wang, W. Chu, L. Huber, T. Tu, Y. Dai, J. Wang, H. Peng, J. Zhao, and X.-Y. Zhu, Proc. Natl. Acad. Sci. U.S.A. **119**, e2122436119 (2022).
[11] I. Bersuker, *The Jahn-Teller Effect* (Cambridge University Press, 2006).
[12] P. A. M. Dirac, Math. Proc. Camb. Philos. Soc. **26**, 361–375 (1930).
[13] J. Frenkel, *Wave mechanics, advanced general theory*, Vol. 1 (Oxford University Press, 1934).
[14] M. Beck, Phys. Rep. **324**, 1–105 (2000).
[15] I. G. Lang and Y. A. Firsov, Zh. Eksp. Teor. Fiz. **45**, 378 (1963), [Sov. Phys. JETP 18, 262 (1964)].
[16] M. Hohenadler and W. von der Linden, "Lang-firsov approaches to polaron physics: From variational methods to unbiased quantum monte carlo simulations," in *Springer Series in Materials Science* (Springer Netherlands, 2007) p. 463–502.
[17] M. Abramowitz and I. A. Stegun, eds., *Handbook of mathematical functions*, Dover Books on Mathematics (Dover Publications, Mineola, NY, 1965).
[18] G. M. Koutentakis, A. Ghazaryan, and M. Lemeshko, Phys. Rev. Res. **5**, 043016 (2023).
[19] A. Alexandrov and J. Devreese, *Advances in Polaron Physics* (Springer Berlin Heidelberg, 2009).
[20] F. Chevy, Phys. Rev. A **74**, 063628 (2006).
[21] I. Hubač and S. Wilson, "Brillouin-wigner perturbation theory," in *Brillouin-Wigner Methods for Many-Body Systems* (Springer Netherlands, Dordrecht, 2010) pp. 37–68.
